# Supplementary material for: Fluctuation-induced phase separation in metric and topological models of collective motion
Source: arXiv:2008.01397 source file (2020-08-04)
Supplement: Supplementary file 1 [file SI_v9.pdf]

# Fluctuation-induced phase-separation scenario in metric and topological models of collective motion.

David Martin,[1] Hugues Chaté,[2] Cesare Nardini,[2] Alexandre Solon,[3] Julien Tailleur,[1] and Frédéric Van Wijland[1]

[1]*Laboratoire Matière et Systèmes Complexes, UMR 7057 CNRS/P7, Université Paris Diderot, 10 rue Alice Domon et Léonie Duquet, 75205 Paris cedex 13, France*

[2]*Service de Physique de l'État Condensé, CNRS UMR 3680, CEA-Saclay, 91191 Gif-sur-Yvette, France*

[3]*Laboratoire Physique théorique de la Matière condensé, Sorbonne Université, 4 place Jussieu, 75252 Paris Cedex 05, France*

(Dated: July 8, 2020 – SI˙v9)

## CONTENTS

I. Linear stability analysis of hydrodynamic equations of metric models 1

II. The fluctuating metric model 2
A. Explicit solution in the high temperature regime 2
B. The low-temperature regime 4

III. The topological model 4
A. Linear stability analysis of mean-field hydrodynamic equations 4
B. Dressing the topological model with noise 5

IV. Simulations 7
A. Stochastic partial differential equations. 7
B. Microscopic models 7

References 7

## I. LINEAR STABILITY ANALYSIS OF HYDRODYNAMIC EQUATIONS OF METRIC MODELS

In this appendix, we show that the homogeneous ordered solutions of the hydrodynamics equations (1) and (2) of the main text are linearly unstable when $\alpha'(\rho) \neq 0$ at the onset of order, i.e for $\alpha = 0^-$ . We start from the mean-field PDEs:

$$\partial_t \rho = D\partial_{xx}\rho - v\partial_x m \tag{1}$$

$$\partial_t m = D\partial_{xx} m - v\partial_x \rho - \alpha(\rho) m - \gamma \frac{m^3}{\rho^2} \tag{2}$$

To simplify the linear stability analysis, we define $x = \tilde{x}D/v$ and $t = \tilde{t}D/v^2$ to eliminate two parameters :

$$\partial_{\tilde{t}} \rho = \partial_{\tilde{x}\tilde{x}}\rho - \partial_{\tilde{x}} m \tag{3}$$

$$\partial_{\tilde{t}} m = \partial_{\tilde{x}\tilde{x}} m - \partial_{\tilde{x}} \rho - \tilde{\alpha}(\rho) m - \tilde{\gamma} \frac{m^3}{\rho^2} \ , \tag{4}$$

where $\tilde{\alpha}(\rho) = D\alpha(\rho)/v^2$ and $\tilde{\gamma} = D\gamma/v^2$. To lighten the notations, we now drop the tilde notation for the rest of this appendix.

The linearized dynamics of perturbations $\delta m$ and $\delta\rho$ around homogeneous solutions $m_0$, $\rho_0$, are given, in Fourier space, by:

$$\partial_t \begin{pmatrix} \delta\rho_q \\ \delta m_q \end{pmatrix} = \begin{pmatrix} -q^2 & -iq \\ -iq - \sqrt{\frac{|\alpha|}{\gamma}}(\alpha'\rho_0 + 2\alpha) & -q^2 + 2\alpha \end{pmatrix} \begin{pmatrix} \delta\rho_q \\ \delta m_q \end{pmatrix} \ , \tag{5}$$

where we used that $m_0 = \rho_0 \sqrt{\frac{|\alpha|}{\gamma}}$. The growth rates of the perturbations are given by the two eigenvalues:

$$\lambda_\pm = \frac{-\left(2q^2 - 2\alpha\right) \pm \sqrt{\Delta}}{2} \tag{6}$$

where $\Delta$ is given by:

$$\Delta = \left(2q^2 - 2\alpha\right)^2 + 4iq\left(iq + \sqrt{\frac{|\alpha|}{\gamma}}\left(\alpha'\rho_0 + 2\alpha\right)\right) - q^2\left(q^2 - 2\alpha\right) \tag{7}$$

The stability of the homogeneous solution is determined by the sign of the real part of the eigenvalues $\lambda^{\pm}$. An unstable eigenvalues exists as soon as $|\Re(2q^2-2\alpha)| < |\Re(\sqrt{\Delta})|$. An instability thus exists as soon as:

$$2\Re(\sqrt{\Delta})^2 - 2\Re\left(2q^2-2\alpha\right)^2 = -a + \sqrt{a^2+b(q)} > 0\ , \tag{8}$$

where $a$ is an unimportant positive term that we do not report and $b(q)$ is given by:

$$b(q) = -\frac{16\alpha q^2}{\gamma}\left(\rho_0\alpha'\left(4\alpha+\rho_0\alpha'\right) - 4\alpha(\alpha(2\gamma-1)-\gamma)\right) - 64\alpha(5\alpha-2)q^4 - 64(-4\alpha+1)q^6 - 64q^8 \tag{9}$$

This expression simplifies as $q \to 0$, leading to

$$b(q) \underset{q\to 0}{\sim} -\frac{16\alpha q^2}{\gamma}\left(\rho_0\alpha'\left(4\alpha+\rho_0\alpha'\right) - 4\alpha(\alpha(2\gamma-1)-\gamma)\right) \tag{10}$$

At the onset of the transition, $\alpha \sim 0$, and $b(q)$ reads

$$b(q) \underset{q\to 0}{\sim} -\frac{16\alpha q^2\rho_0^2}{\gamma}(\alpha')^2 \tag{11}$$

The homogeneous ordered solution is thus unstable close to the onset whenever $\alpha'(\rho_0) \neq 0$. This shows that the mean-field PDEs (1) and (2) with a density-dependent $\alpha(\rho)$ cannot exhibit a continuous transition to collective motion.

## II. THE FLUCTUATING METRIC MODEL

We start from the mean-field dynamics dressed by a Gaussian noise:

$$\partial_t\rho = D\partial_{xx}\rho - \partial_x(vm) \tag{12}$$

$$\partial_t m = D\partial_{xx}m - \partial_x(v\rho) - \alpha m - \gamma\frac{m^3}{\rho^2} + \sqrt{2\sigma\rho}\eta \tag{13}$$

which correspond to Eqs. (1) and (3) of the main text.

We show in this appendix that fluctuations renormalize the hydrodynamic theory and make $\alpha$ density-dependent. More specifically, we derive Eq. (8) of the main text and the corresponding renormalization of $\gamma$. In Section **??**, we do so in the high-temperature regime, where calculations can be done explicitely. We then discuss the low-temperature regime in Section **??**.

### A. Explicit solution in the high temperature regime

Equation (5) of the main text shows that, to order $m_0^3$, the bare value of $\mathcal{F}$ is dressed up by:

$$\frac{1}{2}\frac{\partial^2\mathcal{F}}{\partial^2 m}\langle\delta m^2\rangle + \frac{1}{2}\frac{\partial^2\mathcal{F}}{\partial^2\rho}\langle\delta\rho^2\rangle + \frac{\partial^2\mathcal{F}}{\partial m\partial\rho}\langle\delta\rho\delta m\rangle = 3\gamma\frac{m_0}{\rho_0^2}\langle\delta m^2\rangle + 3\gamma\frac{m_0^3}{\rho_0^4}\langle\delta\rho^2\rangle - 6\gamma\frac{m_0^2}{\rho_0^3}\langle\delta m\delta\rho\rangle\ . \tag{14}$$

We thus need to compute $\langle\delta m^2\rangle$ up to order $m_0^2$, $\langle\delta m\delta\rho\rangle$ up to order $m_0$ and $\langle\delta\rho^2\rangle$ up to $\mathcal{O}(1)$. Going into Fourier space, the linear Gaussian dynamics of $\delta\rho$ and $\delta m$ given by Eqs (6) and (7) of the main text read:

$$\partial_t\begin{pmatrix}\delta\rho_q\\ \delta m_q\end{pmatrix} = \begin{pmatrix}-Dq^2 & -ivq\\ M_{21}^q & M_{22}^q\end{pmatrix}\begin{pmatrix}\delta\rho_q\\ \delta m_q\end{pmatrix} + \begin{pmatrix}0\\ \sqrt{2\sigma\rho_0}\eta_q\end{pmatrix}\ , \tag{15}$$

where $\eta_q$ is the fourier transform of the Gaussian white noise with correlations $\langle\eta_q(t)\eta_{q'}(t')\rangle = \delta_{q+q',0}\delta(t-t')$ and the matrix coefficients $M_{21}$, $M_{22}$ are given by:

$$M_{22}^q = -Dq^2 - \alpha - 3\gamma\frac{m_0^2}{\rho_0^2} \tag{16}$$

$$M_{21}^q = -iqv + 2\gamma\frac{m_0^3}{\rho_0^3} \tag{17}$$

Since we are interested in the equal-time two-point correlation functions in the steady-state, we can use Itō calculus on the stochastic system (15) to get the following closed system of equations:

$$0 = (M^q_{11} + M^{q'}_{11})\langle\delta\rho_q\delta\rho_{q'}\rangle + M^q_{12}\langle\delta m_q\delta\rho_{q'}\rangle + M^{q'}_{12}\langle\delta\rho_q\delta m_{q'}\rangle \tag{18}$$
$$0 = (M^q_{22} + M^{q'}_{11})\langle\delta m_q\delta\rho_{q'}\rangle + M^q_{21}\langle\delta\rho_q\delta\rho_{q'}\rangle + M^{q'}_{12}\langle\delta m_q\delta m_{q'}\rangle \tag{19}$$
$$0 = (M^q_{22} + M^{q'}_{22})\langle\delta m_q\delta m_{q'}\rangle + M^q_{21}\langle\delta\rho_q\delta m_{q'}\rangle + M^{q'}_{21}\langle\delta m_q\delta\rho_{q'}\rangle + \sigma\rho_0\delta_{q+q',0} \tag{20}$$

Solving this system in the regime $\alpha > 0$ yields:

$$\langle\delta m_q\delta m_{-q}\rangle = \sigma\rho_0\Bigg[\frac{2D^2q^2+\alpha D+v^2}{2\left(2Dq^2+\alpha\right)\left(D^2q^2+\alpha D+v^2\right)} - \frac{3\gamma\left(2D^2q^2+\alpha D+vDq+v^2\right)\left(2D^2q^2+D(\alpha-qv)+v^2\right)}{2\left(\alpha+2Dq^2\right)^2\left(D^2q^2+\alpha D+v^2\right)^2}\frac{m_0^2}{\rho_0^2}\Bigg] + O\left(m_0^3\right) \tag{21}$$
$$\langle\delta\rho_q\delta\rho_{-q}\rangle = \frac{\sigma\rho_0 v^2}{2\left(2Dq^2+\alpha\right)\left(D^2q^2+\alpha D+v^2\right)} + O\left(m_0^2\right) \tag{22}$$
$$\langle\delta m_q\delta\rho_{-q}\rangle = \frac{i\rho_0\sigma vDq}{2\left(2Dq^2+\alpha\right)\left(D^2q^2+\alpha D+v^2\right)} + O\left(m_0^2\right) \tag{23}$$

Going back to the correlators in real space then gives:

$$\langle\delta m^2\rangle = \int\frac{dq}{2\pi}\langle\delta m_q\delta m_{-q}\rangle = \sigma\rho_0\frac{v^2\sqrt{\frac{2\alpha}{D}}+\alpha\sqrt{v^2+\alpha D}}{8\alpha v^2+4\alpha^2 D} - \sigma\rho_0\frac{3\gamma D\left(\frac{\alpha D}{\sqrt{v^2+\alpha D}}+\frac{\sqrt{2}v^2\left(2v^2+3\alpha D\right)}{(\alpha D)^{3/2}}\right)}{8\left(\alpha D+2v^2\right)^2}\frac{m_0^2}{\rho_0^2} + O(m_0^3) \tag{24}$$
$$\langle\delta\rho^2\rangle = \int\frac{dq}{2\pi}\langle\delta\rho_q\delta\rho_{-q}\rangle = \sigma\rho_0\frac{v^2\left(\sqrt{\frac{2\alpha}{D}}-\frac{\alpha}{\sqrt{v^2+\alpha D}}\right)}{4\alpha\left(\alpha D+2v^2\right)} + O(m_0^2) \tag{25}$$
$$\langle\delta\rho\delta m\rangle = \int\frac{dq}{2\pi}\langle\delta\rho_q\delta m_{-q}\rangle = 0 + O(m_0^2) \tag{26}$$

The equation (5) of the main text can now be rewritten in a closed form as:

$$\partial_t m_0 = D\partial_{xx}m_0 - v\partial_x m_0 - \tilde{\alpha}(\rho_0)m_0 - \tilde{\gamma}(\rho_0)\frac{m_0^3}{\rho_0^2} \tag{27}$$

with the dressed coefficent $\tilde{\gamma}(\rho_0)$ and $\tilde{\alpha}(\rho_0)$ given by:

$$\tilde{\gamma}(\rho_0) = \gamma + \frac{3\sigma\gamma}{4v\rho_0}\frac{\sqrt{\frac{2v^2}{D\alpha}}-\frac{1}{\sqrt{1+\frac{\alpha D}{v^2}}}}{\frac{\alpha D}{v^2}+2} - \frac{9\sigma\gamma^2 D}{8v^3\rho_0}\frac{\left(\frac{\alpha D}{v^2\sqrt{1+\frac{\alpha D}{v^2}}}+\frac{\sqrt{2}\left(2+3\frac{\alpha D}{v^2}\right)}{\left(\frac{\alpha D}{v^2}\right)^{3/2}}\right)}{\left(\frac{\alpha D}{v^2}+2\right)^2} = \gamma + \frac{\sigma\gamma}{\rho_0 v}f_1\left(\frac{\alpha D}{v^2},\frac{\gamma}{\alpha}\right) \tag{28}$$
$$\tilde{\alpha}(\rho_0) = \alpha + \frac{\sigma\gamma}{\rho_0 v}\frac{\sqrt{\frac{18v^2}{D\alpha}}+3\sqrt{1+\frac{D\alpha}{v^2}}}{8+4\frac{D\alpha}{v^2}} = \alpha + \frac{\sigma\gamma}{\rho_0 v}\,f\left(\frac{D\alpha}{v^2}\right) \tag{29}$$

### B. The low-temperature regime

In the low temperature regime, the correlators (21), (22) and (23) read :

$$\langle \delta m_q \delta m_{-q} \rangle = \frac{1}{\alpha} \frac{a_1\left(\frac{\sqrt{D}q}{\sqrt{\alpha}}, \frac{m_0}{\rho_0}, \frac{\gamma}{\alpha}, \frac{v^2}{\alpha D}\right)}{h\left(\frac{\sqrt{D}q}{\sqrt{\alpha}}, \frac{m_0}{\rho_0}, \frac{\gamma}{\alpha}, \frac{v^2}{\alpha D}\right)} \tag{30}$$

$$\langle \delta \rho_q \delta \rho_{-q} \rangle = \frac{1}{\alpha} \frac{v^2}{\alpha D} \frac{a_2\left(\frac{\sqrt{D}q}{\sqrt{\alpha}}, \frac{m_0}{\rho_0}, \frac{\gamma}{\alpha}, \frac{v^2}{\alpha D}\right)}{h\left(\frac{\sqrt{D}q}{\sqrt{\alpha}}, \frac{m_0}{\rho_0}, \frac{\gamma}{\alpha}, \frac{v^2}{\alpha D}\right)} \tag{31}$$

$$\langle \delta m_q \delta \rho_{-q} \rangle = \frac{1}{\alpha} \frac{v^2}{\alpha D} \frac{a_3\left(\frac{\sqrt{D}q}{\sqrt{\alpha}}, \frac{m_0}{\rho_0}, \frac{\gamma}{\alpha}, \frac{v^2}{\alpha D}\right)}{h\left(\frac{\sqrt{D}q}{\sqrt{\alpha}}, \frac{m_0}{\rho_0}, \frac{\gamma}{\alpha}, \frac{v^2}{\alpha D}\right)} \tag{32}$$

Where the expressions of $a_1$, $a_2$, $a_3$ and $h$ are given by:

$$h\left(\tilde{q}, u, v, w\right) = 2(2\tilde{q}+1)(\tilde{q}^2+w+1) + 6u^2v(2\tilde{q}+1)(4\tilde{q}^2+2w+3) + 18u^4v^2(5\tilde{q}+w+3) + 2u^6v^2(27v-4w)$$
$$a_1\left(\tilde{q}, u, v, w\right) = (3u^2v+1+2\tilde{q}^2)(3u^2v+1+w+2\tilde{q}^2)$$
$$a_2\left(\tilde{q}, u, v, w\right) = 3u^2v+1+2\tilde{q}^2$$
$$a_3\left(\tilde{q}, u, v, w\right) = 2u^3v + \frac{3i}{\sqrt{w}}u^2v\tilde{q} + \frac{i}{\sqrt{w}}\tilde{q}(2\tilde{q}^2+1)$$

The renormalized Landau term can still be formally computed using the integral expressions (24)-(26), even though the latter cannot be carried out explicitly, unlike in the high temperature regime.

## III. THE TOPOLOGICAL MODEL

### A. Linear stability analysis of mean-field hydrodynamic equations

We recall the definition of our topological mean-field model:

$$\partial_t \rho = D\nabla^2\rho - v\nabla m \tag{33}$$

$$\partial_t m = D\nabla^2 m - v\nabla\rho + 2\Gamma\rho\beta\bar{m}\left(1+\frac{\beta^2\bar{m}^2}{6}\right) - 2\Gamma m\left(1+\frac{\beta^2}{2}\bar{m}^2\right) \tag{34}$$

$$\bar{m} = \frac{1}{k}\int_{x-y(x)}^{x+y(x)} m(x)dx \tag{35}$$

where $y(x)$ is defined implicitly through $k = \int_{x-y(x)}^{x+y(x)} \rho(x)dx$.

We study the linear stability of homogeneous solutions $\rho = \rho_0$ , $m = m_0$ of Eqs. (33) and (34). Note that the fluctuations $\delta\rho$ and $\delta m$ will also lead to $y(x) = y_0 + \delta y(x)$. We first determine how the non local term $\bar{m}$ is impacted by the perturbations $\delta\rho$, $\delta m$ and $\delta y$. To first order,

$$\bar{m} = \frac{\int_{x-y_0-\delta y}^{x+y_0+\delta y}(m_0+\delta m(z))dz}{k} = \int_{x-y_0}^{x+y_0}\frac{\delta m(z)dz}{k} + 2\delta y\frac{m_0}{k} \tag{36}$$

We can relate $\delta y$ to $\delta\rho$ by using the implicit equation $k = \int_{x-y(x)}^{x+y(x)} \rho(x)dx$ :

$$\delta y = -\tfrac{1}{2\rho_0}\int_{x-y_0}^{x+y_0}\delta\rho(z)dz \tag{37}$$

Interestingly, the fluctuations of $\rho$ impact $\bar{m}$, despite the topological nature of the latter, through $\delta y$. Using (36) and (37), we obtain the closed linearized dynamics obeyed by $\delta\rho$ and $\delta m$ in Fourier space:

$$\begin{pmatrix}\delta\dot{\rho}_q \\ \delta\dot{m}_q\end{pmatrix} = \begin{pmatrix}-Dq^2 & -ivq \\ M_{21}^q & M_{22}^q\end{pmatrix}\begin{pmatrix}\delta\rho_q \\ \delta m_q\end{pmatrix} , \tag{38}$$

where the matrix coefficients $M_{21}$ and $M_{22}$ are given by:

$$M_{12}^q = \frac{\Gamma}{3}\left(\frac{\beta m_0}{\rho_0}\right)^3 + 2\Gamma\beta\frac{m_0}{\rho_0} - iqv + \Gamma\,\text{sinc}(qy_0)\frac{m_0}{\rho_0}\left(\left(\frac{\beta m_0}{\rho_0}\right)^2(-\beta+2) - 2\beta\right) \tag{39}$$

$$M_{22}^q = -2\Gamma - \Gamma\left(\frac{\beta m_0}{\rho_0}\right)^2 + \Gamma\,\text{sinc}(qy_0)\left(\left(\frac{\beta m_0}{\rho_0}\right)^2(\beta-2) + 2\beta\right) - Dq^2 \tag{40}$$

We are interested in the onset of the transition where $m_0$ is small and $\beta = 1 + o(m_0)$. At leading order in $m_0$, the matrix coefficients then simplify into:

$$M_{12}^q = -iqv + O(m_0) \tag{41}$$

$$M_{22}^q = 2\Gamma\left(\text{sinc}(qy_0) - 1\right) - Dq^2 + O(m_0) \tag{42}$$

Within this regime, the eigenvalues of the dynamic are :

$$\lambda_\pm = \frac{-\left(2Dq^2 + 2\Gamma\left(1 - \text{sinc}(qy_0)\right)\right) \pm \sqrt{\Delta}}{2}\,, \tag{43}$$

with the discriminant $\Delta$ being given by:

$$\Delta = \left(2Dq^2 + 2\Gamma\left(1 - \text{sinc}(qy_0)\right)\right)^2 - 4v^2q^2 + Dq^2\left(Dq^2 + 2\Gamma\left(1 - \text{sinc}(qy_0)\right)\right)\ . \tag{44}$$

As in the previous subsection, an instability emerges when

$$2\Re(\sqrt{\Delta})^2 - 2\Re\left(2Dq^2 + 2\Gamma\left(1 - \text{sinc}(qy_0)\right)\right)^2 = -a + \sqrt{a^2 + b(q)} > 0 \tag{45}$$

In Eq. (45), $a$ is again an unimportant positive term and the stability is determined by the sign of $b(q)$ whose expression reads:

$$\begin{aligned}\frac{b(q)}{64q^2} = &-\Gamma^2\left(\text{sinc}(qy_0) - 1\right)^2\left(v^2 + 2D\left(1 - \text{sinc}(qy_0)\right)\right) - q^2D\Gamma\left(1 - \text{sinc}(qy_0)\right)\left(5D\Gamma\left(1 - \text{sinc}(qy_0)\right) + 2v^2\right)\\ &-D^2q^4\left(4D\Gamma\left(1 - \text{sinc}(qy_0)\right) + v^2\right) - D^4q^6\end{aligned} \tag{46}$$

All the terms in (46) are negative; the homogeneous ordered solution is thus always stable at onset. Our topological field theory (33)-(34) thus predicts, at mean-field order, a continuous transition.

### B. Dressing the topological model with noise

We now add a small gaussian noise $\sqrt{2\sigma\rho}\,\eta$ to (34), as described in the main text, and determine the renormalization of the linear aligning term in $\mathcal{F}_{\text{topo}}$. Following the main text, we define the hydrodynamic fields

$$\rho_0 = \langle\rho(x,t)\rangle \qquad m_0 = \langle m(x,t)\rangle \qquad y_0 = \langle y(x,t)\rangle \tag{47}$$

and the corresponding fluctuations

$$\delta\rho = \rho(x,t) - \langle\rho(x,t)\rangle \qquad \delta m = m(x,t) - \langle m(x,t)\rangle \qquad \delta y = y(x,t) - \langle y(x,t)\rangle \tag{48}$$

As for the metric model, we need to evaluate the non-linearities in $\mathcal{F}_{\text{topo}}$ to second order in $\delta m$, $\delta y$, $\delta\rho$. Within the context of the Landau expansion, we only need the expression of these nonlinearities up to first order in $m_0$ [1]. Within these approximations, the contribution of fluctuations to $\mathcal{F}_{\text{topo}}$ reads:

$$\begin{aligned}\langle\Delta\mathcal{F}_{\text{topo}}\rangle &= \langle\mathcal{F}_{\text{topo}}(\rho_0 + \delta\rho, m_0 + \delta m, y_0 + \delta y)\rangle - \mathcal{F}_{\text{topo}}(\rho_0, m_0, y_0)\\ &\simeq 2\frac{\Gamma\beta}{k}\left\langle\delta\rho(x)\int_{x-y_0}^{x+y_0}\delta m(z)dz\right\rangle + 2\frac{\Gamma\beta}{k}\rho_0\langle\delta y(x)\delta m(x+y_0)\rangle + 2\frac{\Gamma\beta}{k}\rho_0\langle\delta y(x)\delta m(x-y_0)\rangle\\ &\quad + m_0\Gamma\left(\frac{\beta}{k}\right)^2(\beta-1)\left\langle\left(\int_{x-y_0}^{x+y_0}\delta m(z)dz\right)^2\right\rangle - \Gamma\left(\frac{\beta}{k}\right)^2(4m_0y_0)\left\langle\delta m(x)\int_{x-y_0}^{x+y_0}\delta m(z)dz\right\rangle\\ &\quad + 4m_0\frac{\Gamma\beta}{k}\langle\delta\rho(x)\delta y(x)\rangle + O(m_0^2)\end{aligned} \tag{49}$$

We now have to evaluate the expression of the correlators in (49). To do so, we work at the Gaussian, linear level, at which the dynamics of the stochastic fields $\delta\rho$, $\delta m$ read, in Fourier space,

$$\begin{pmatrix} \partial_t \delta\rho_q \\ \partial_t \delta m_q \end{pmatrix} = \begin{pmatrix} -Dq^2 & -ivq \\ M_{21}^q & M_{22}^q \end{pmatrix} \begin{pmatrix} \delta\rho_q \\ \delta m_q \end{pmatrix} + \begin{pmatrix} 0 \\ \sqrt{2\sigma\rho_0}\,\eta_q \end{pmatrix} , \tag{50}$$

where $\eta_q$ is the fourier transform of the Gaussian white noise, with correlations $\langle \eta_q \eta_{q'} \rangle = \delta_{q+q',0}$, and the matrix coefficients $M_{21}^q$, $M_{22}^q$ are given by (39), (40). Using Ito Calculus, the correlators satisfy in the steady state:

$$0 = (M_{11}^q + M_{11}^{q'})\langle \delta\rho_q \delta\rho_{q'} \rangle + M_{12}^q \langle \delta m_q \delta\rho_{q'} \rangle + M_{12}^{q'} \langle \delta\rho_q \delta m_{q'} \rangle \tag{51}$$

$$0 = (M_{22}^q + M_{11}^{q'})\langle \delta m_q \delta\rho_{q'} \rangle + M_{21}^q \langle \delta\rho_q \delta\rho_{q'} \rangle + M_{12}^{q'} \langle \delta m_q \delta m_{q'} \rangle \tag{52}$$

$$0 = (M_{22}^q + M_{22}^{q'})\langle \delta m_q \delta m_{q'} \rangle + M_{21}^q \langle \delta\rho_q \delta m_{q'} \rangle + M_{21}^{q'} \langle \delta m_q \delta\rho_{q'} \rangle + \sigma\rho_0 \delta_{q+q',0} \tag{53}$$

Solving this system at first order in $m_0$ then yields:

$$\langle \delta m_q \delta m_{-q} \rangle = \sigma\rho_0 \frac{2D\Gamma - 2D\Gamma\beta\,\mathrm{sinc}(qy_0) + 2D^2q^2 + v^2}{4(\Gamma - \Gamma\beta\,\mathrm{sinc}(qy_0) + Dq^2)\,(2D\Gamma - 2D\Gamma\beta\,\mathrm{sinc}(qy_0) + D^2q^2 + v^2)} + O\left(m_0^2\right) \tag{54}$$

$$\langle \delta\rho_q \delta\rho_{-q} \rangle = \frac{\sigma\rho_0 v^2}{4(\Gamma - \Gamma\beta\,\mathrm{sinc}(qy_0) + Dq^2)\,(2D\Gamma - 2D\Gamma\beta\,\mathrm{sinc}(qy_0) + D^2q^2 + v^2)} + O\left(m_0^2\right) \tag{55}$$

$$\begin{aligned} \langle \delta m_q \delta\rho_{-q} \rangle = & \frac{iqDv\sigma\rho_0}{4(\Gamma - \Gamma\beta\,\mathrm{sinc}(qy_0) + Dq^2)\,(2D\Gamma - 2D\Gamma\beta\,\mathrm{sinc}(qy_0) + D^2q^2 + v^2)} \\ & + \frac{\beta\sigma v^2 \Gamma\,(1 - \mathrm{sinc}\,(qy_0))\, m_0}{4\,(\Gamma - \Gamma\beta\,\mathrm{sinc}\,(qy_0) + Dq^2)^2\,(2D\Gamma - 2D\Gamma\beta\,\mathrm{sinc}\,(qy_0) + D^2q^2 + v^2)} + O\left(m_0^2\right) \end{aligned} \tag{56}$$

We are now in position to compute $\langle \Delta\mathcal{F}_{\mathrm{topo}} \rangle$ in (49). After a lengthy but straightforward computation we find :

$$\langle \Delta\mathcal{F}_{\mathrm{topo}} \rangle = \frac{m_0\Gamma}{\rho_0}\sigma \left[2\beta(c_4 - c_1) - \beta^2(1-\beta)c_2 - 2\beta^2 c_3\right] + O(m_0^2) \tag{57}$$

Where $c_1, ..., c_4$ are given by:

$$c_1 = \int \frac{dq}{2\pi} \frac{v^2\,\mathrm{sinc}(qy_0)}{4(\Gamma - \Gamma\beta\,\mathrm{sinc}(qy_0) + Dq^2)\,(2D\Gamma - 2D\Gamma\beta\,\mathrm{sinc}(qy_0) + D^2q^2 + v^2)} \tag{58}$$

$$c_2 = \int \frac{dq}{2\pi} \frac{\mathrm{sinc}^2(qy_0)\left[2D\Gamma - 2D\Gamma\beta\,\mathrm{sinc}(qy_0) + 2D^2q^2 + v^2\right]}{4(\Gamma - \Gamma\beta\,\mathrm{sinc}(qy_0) + Dq^2)\,(2D\Gamma - 2D\Gamma\beta\,\mathrm{sinc}(qy_0) + D^2q^2 + v^2)} \tag{59}$$

$$c_3 = \int \frac{dq}{2\pi} \frac{\mathrm{sinc}(qy_0)\left[2D\Gamma - 2D\Gamma\beta\,\mathrm{sinc}(qy_0) + 2D^2q^2 + v^2\right]}{4(\Gamma - \Gamma\beta\,\mathrm{sinc}(qy_0) + Dq^2)\,(2D\Gamma - 2D\Gamma\beta\,\mathrm{sinc}(qy_0) + D^2q^2 + v^2)} \tag{60}$$

$$c_4 = \int \frac{dq}{2\pi} \frac{\beta v^2\,(\Gamma - \Gamma\,\mathrm{sinc}\,(qy_0))\,\mathrm{sinc}(qy_0)\,(1 - \cos(qy_0))}{4\,(\Gamma - \Gamma\beta\,\mathrm{sinc}\,(qy_0) + Dq^2)^2\,(2D\Gamma - 2D\Gamma\beta\,\mathrm{sinc}\,(qy_0) + D^2q^2 + v^2)} \tag{61}$$

$$\tag{62}$$

Making these integrals dimension-free leads to a scaling form

$$\langle \Delta\mathcal{F}_t \rangle = \frac{2\sigma m_0 \Gamma}{k} f\left(\beta, \frac{\Gamma k}{v\rho_0}, \frac{\Gamma D}{v^2}\right) \tag{63}$$

The expression of $g$ in Eq.(12) of the main text then stems from (57) as :

$$g\left(\beta, \frac{\Gamma k}{v\rho_0}, \frac{\Gamma D}{v^2}\right) = \frac{\beta(c_1 - c_4)}{\rho_0} + \frac{\beta^2(1-\beta)}{2\rho_0}c_2 + \frac{\beta^2 c_3}{\rho_0} \tag{64}$$

Importantly, the dependence of $f$ on $\rho_0$ cannot be eliminated, so that the renormalization of the critical-temperature indeed leads to a density-dependent onset of order. In the high temperature phase where $0 < \beta < 1$, it can be shown that $c_1 > c_4$, and that $c_1$, $c_2$, $c_3$ are positive. Thus, $f$ is a density-dependent positive function in this region, which lowers the critical temperature.

The renormalization of Eqs. (33) and (34) thus suggest a discontinuous transition to collective motion. This is confirmed upon simulating the SPDE (1) and (3) of the main text, in which $\mathcal{F}$ has been replaced by $\mathcal{F}_{\mathrm{topo}}$: close to the onset, we indeed observe a regime where coexistence occurs between dense polar bands and a disordered homogeneous background (See Fig. 1).

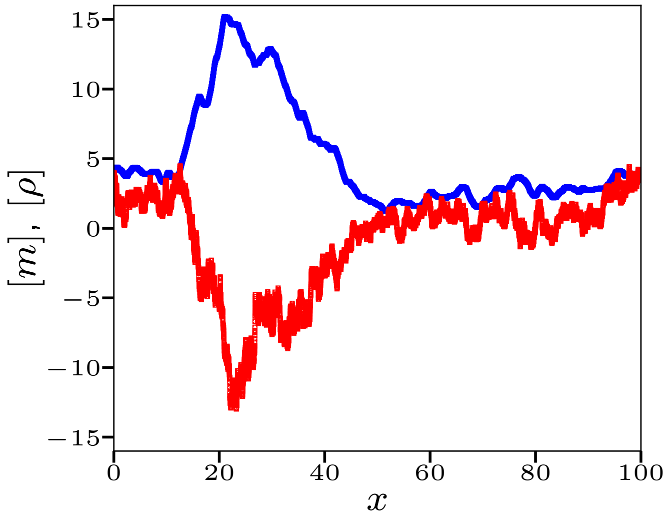


FIG. 1. Snapshot of a numerical integration of (33) and (34) supplemented with a Gaussian white noise $\sqrt{\sigma\rho}\eta$. The magnetization (red) and the density (blue) fields show a dense polar band propagating in a disordered gas. Parameters: $D = \Gamma = v = 1$, $k = 0.5$, $\rho_0 = 5$, $L = 100$, $\beta = 1.1$, $dx = 0.01$, $dt = 0.01$, $\sigma = 0.4$.

## IV. SIMULATIONS

### A. Stochastic partial differential equations.

The numerical integrations of the stochastic PDEs were carried out using a semi-spectral method with a semi-implicit Euler scheme. At every time step, the Gaussian noise fields are drawn in direct space. The latter being discretized, at every lattice site, one draws a Gaussian random number of zero mean and variance $\sqrt{\frac{2Ddt}{dx}}$. All the non-linearities are also computed in direct space. All fields are then Fourier-transformed to $q$-space, where the time-stepping takes place. Anti-aliasing with the standard 3/2 rule was carried out after time-stepping.

### B. Microscopic models

The simulations of the microscopic models rely on a parallel update of all particles. Each spin $s$ has a probability $W(s)dt$ to flip during a time-step $dt$. The positions of the particles are then evolved using a forward Euler scheme to integrate the Langevin dynamics.

---

[1] Note that, were we to also look for the dressed coefficient $\tilde{\gamma}$, we would have had to go up to order $m_0^3$ instead; this is beyond the scope of this paper.
